# Supplementary material for: Limitations of Time Resources in Human Relationships Determine Social Structures
Source: arXiv:1605.07305 source file (2017-02-14)
Supplement: Supplementary file 1 [file si.pdf]

## **Supplementary Materials:**

# Limitations of Time Resources in Human Relationships Determine Social Structures

Masanori Takano<sup>1,\*</sup> and Ichiro Fukuda<sup>1</sup>

<sup>1</sup>CyberAgent, Inc.

\*takano\_masanori@cyberagent.co.jp.

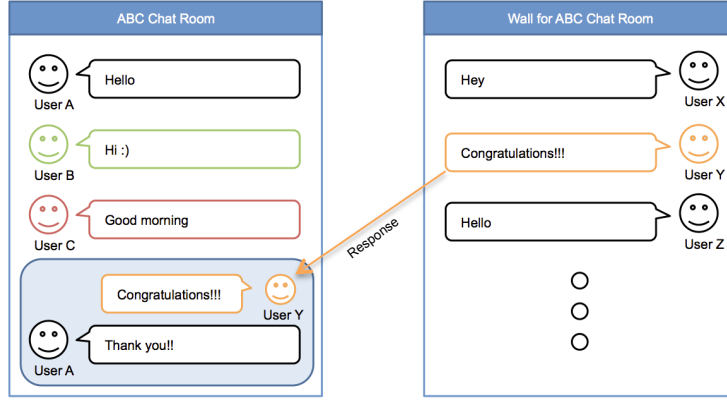

Figure 1: The basic specification of 755, published by 7gogo, Inc. Users have two roles, namely chat member (User A, B and C) or commenter (User X, Y and Z). This application provides two types of interactions, those between chat members and those between chat members and commenters. We term the former a group chat and the latter a wall communication. We treat these as different data sets. Users can perform either role at any time. A chat member creates chat rooms where they chat with other chat members (this is an interaction between chat members). To join a chat room as a chat member, users have to be invited by other chat members. On the other hand, all users can read all chat rooms, and they can post comments to chat rooms as commenters, without limits. Comments are limited to 200 characters (almost all users use Japanese); in contrast, chat members' posts can use unlimited number of characters. Chat members can respond to comments (an interaction between chat members and commenters); however, other users can only read the comments. That is, wall communications are open platforms where users can talk to someone they do not know. On the other hand, group chats are semi-closed platforms where users can speak with acquaintances who were invited by chat members.

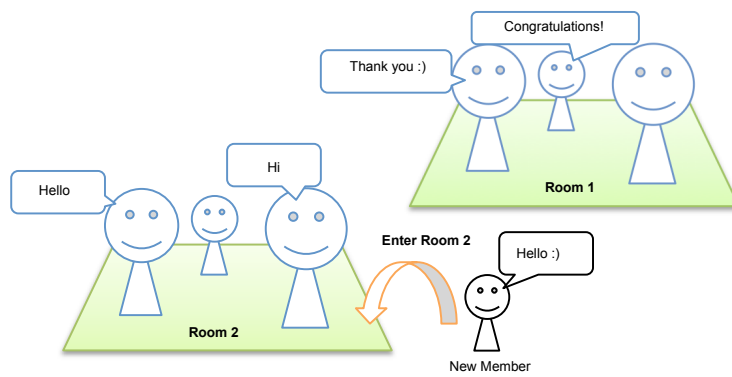

Figure 2: The basic specification of the avatar chat Ameba Pigg, published by CyberAgent, Inc. Users chat in a room where more than one user can belong. They can enter or leave the room any time. Their utterances are limited to 37 characters (almost all users use Japanese), and an unlimited number of utterances can be used. That is, users can talk to anyone at any time.
